# Supplementary material for: Observation of quantum-field-theory dynamics on a spin-phonon quantum computer
Source: arXiv:2509.11477 source file (2025-09-14)
Supplement: Supplementary file 1 [file supplement.pdf]

Supplementary Information on:  
**Observation of quantum-field-theory dynamics on a  
spin-phonon quantum computer**

Anton T. Than, Saurabh V. Kadam, Vinay Vikramaditya, Nhung H. Nguyen, Xingxin Liu,  
Zohreh Davoudi, Alaina M. Green, and Norbert M. Linke

This Supplemental Information contains details on the gate calibrations performed in the experimental implementation of Yukawa dynamics in the main text, along with explicit quantum circuits and their associated parameters for each Trotter step of evolution. We conclude with a discussion of boson-truncation errors in numerical simulations of the time dynamics and an assessment of the numerical convergence.

## I. EXPERIMENTAL CALIBRATION

### A. Motional-mode frequency

Electronic interference causes variations in the trap potential, causing the motional-mode frequency to drift over time. To mitigate drift on the timescale of an hour, we calibrate the motional-mode frequency approximately every 20 minutes using the method described in Ref. [1].

In addition to long-term drifts, the motional-mode frequency has an oscillation at 180 Hz, likely due to electronic interference from the 60 Hz AC line. To mitigate this error, we trigger the start of the experiment on the AC line and ensure that the circuit sequence falls within a period where the motional mode frequency is stable.

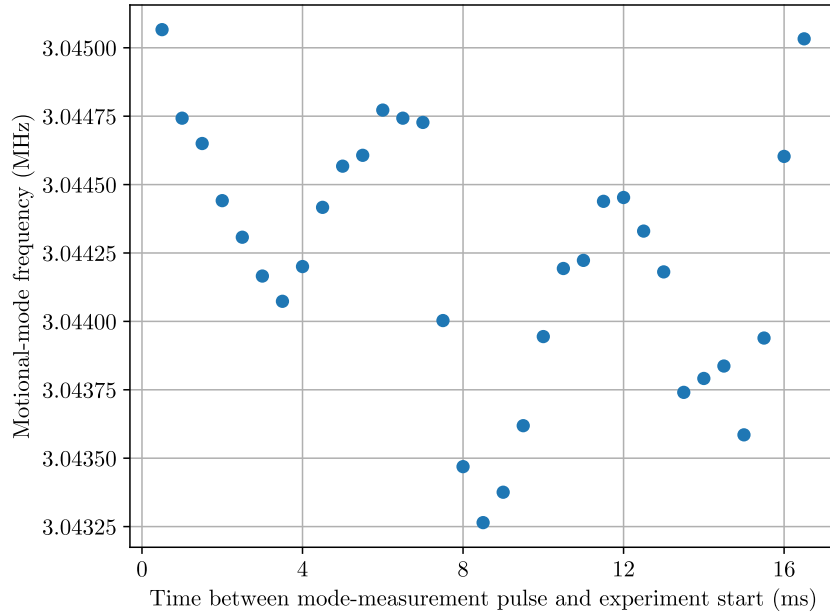

FIG. 1. Motional-mode-frequency variation over time within one 60 Hz cycle. The signal shows a strong oscillation at 180 Hz. To mitigate errors from this variation, we trigger the start of the experiment on the AC line, and start the circuit sequence at 14 ms where the motional-mode variation is small.

## B. Single-qubit and entangling gates

Single-qubit and entangling gates are routinely calibrated approximately every 20 minutes to account for drifts in Raman-beam power and alignment. For single-qubit gates, we calibrate the time it takes to perform an  $R_j^X(\pi/2) = e^{-i\pi\sigma_j^x/4}$  rotation on each qubit  $j$ . For entangling gates, we calibrate the power it takes to perform an  $MS_{i,j}(\pi/2) = e^{-i\pi\sigma_i^x\sigma_j^x/4}$  rotation on the desired pair of qubits  $i, j$ .

## C. Spin-phonon gate

Spin-phonon gates are implemented by performing a spin-dependent kick operation, described by the unitary

$$\text{SNP}_{j,m}(\eta_{m,j}\Omega_j t, 0) = e^{-i\eta_{m,j}\Omega_j\sigma_j^y(a_m + a_m^\dagger)t/2}, \quad (1)$$

where  $m$  is the mode index,  $j$  is the ion index,  $t$  is the duration of the applied pulse,  $\Omega_j$  is the carrier Rabi frequency on ion  $j$ ,  $\sigma_j^y$  is the Pauli-Y matrix on ion  $j$ ,  $a_m$  ( $a_m^\dagger$ ) is the bosonic annihilation (creation) operator, and  $\eta_{m,j}$  is the Lamb-Dicke parameter, which describes the strength of the ion-mode coupling. When applying the SNP operation to state  $|0\rangle|0\rangle$  (where the first ket denotes the spin- $j$  state and the second denotes the motional-mode- $m$  state), the resulting state is

$$\text{SNP}_{j,m}(\eta_{m,j}\Omega_j t, 0) |0\rangle|0\rangle = \frac{1}{\sqrt{2}} (|+\rangle|\alpha(t)\rangle + |-\rangle|-\alpha(t)\rangle), \quad (2)$$

where  $|\pm\rangle$  are the  $\pm 1$  eigenstates of the  $\sigma^y$  operator, and  $|\pm\alpha(t)\rangle$  is a coherent state with  $\alpha(t) = \eta_{m,j}\Omega_j t/2$ . The probability of measuring this state in spin-state  $|1\rangle$  is

$$P_{|1\rangle}(t) = \frac{1}{2}(1 - e^{-2\alpha^2(t)}). \quad (3)$$

We do a fit to determine the quantity  $\eta_{m,j}\Omega_j$  and use this to calculate the time to apply the spin-phonon gate  $\text{SNP}_{j,m}(\theta, \varphi)$ .

## II. QUANTUM CIRCUITS FOR TROTTERIZED EVOLUTION

The schematic of each step of the Trotterized time evolution in the Yukawa model for the  $N = 2$  and  $N = 4$  systems are presented in the main text. Here, we display the circuits again along with the associated gate angles for completeness. For the symbols and associated unitary operations, see Fig. 1 of the main text.

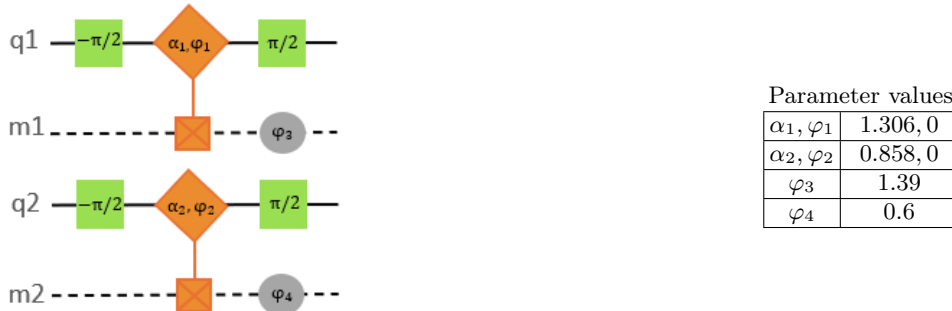

FIG. 2. Circuit diagram for one Trotter step of evolution for  $N = 2$ . While the circuit is composed of two disjoint parts, we run both subcircuits simultaneously on a two-qubit two-phonon system. Gate angles are given in the table to the right.

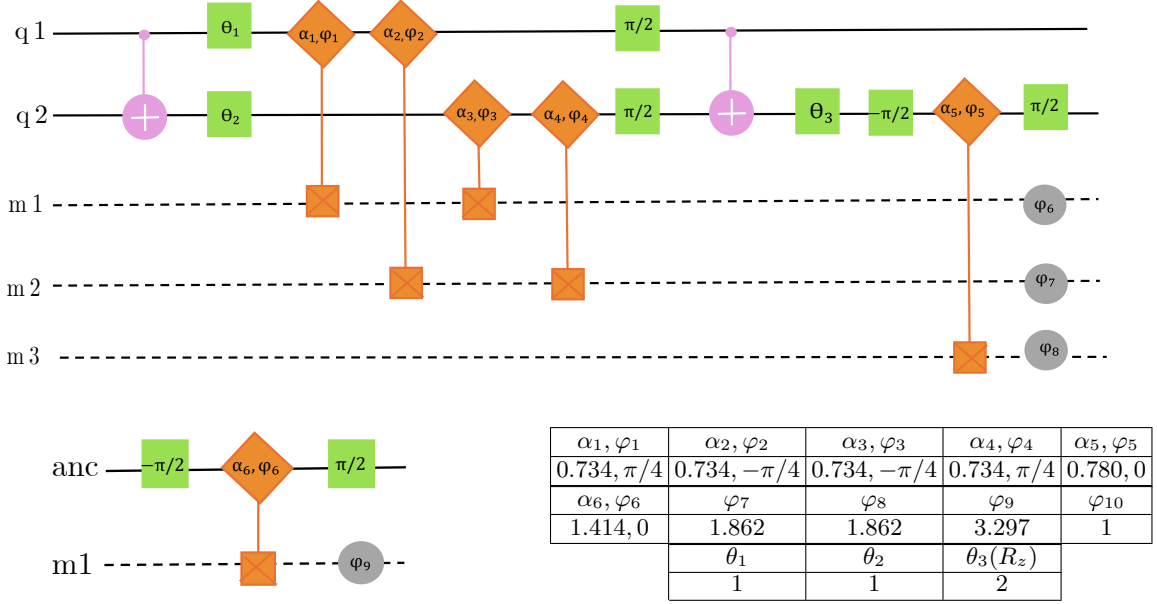

FIG. 3. Circuit diagram for one Trotter step of evolution for  $N = 4$ . To obtain results for a desired simulation time, we run two independent circuits; one with two qubits and three motional modes, and another with one qubit and one motional mode, allowing for each circuit to fit on a three-ion chain. Gate angles are given in the accompanying table.

### III. CLASSICAL SIMULATIONS

#### A. Exact evolution and convergence with bosonic mode cutoff

Classical simulations of continuous-time evolution were performed using exact matrix exponentiation to compute the time-evolution operator. While a large cutoff was used for  $N = 2$ , the simulations became more costly for the  $N = 4$  case as the cutoff increased. To ensure numerical convergence has been achieved in the latter case, we varied bosonic mode cutoff from  $\Lambda = 2$  to  $\Lambda = 8$  and assessed convergence of the mean bosonic-mode occupation. The relative percentage change of this observable, when  $\Lambda$  is decreased in steps of one, was recorded, and its maximum value over the simulation duration was extracted. Mode 2, the highest populated mode, exhibited the largest variation, with the maximum percentage deviation decreasing sharply as  $\Lambda$  is increased, as illustrated in Fig. 4.

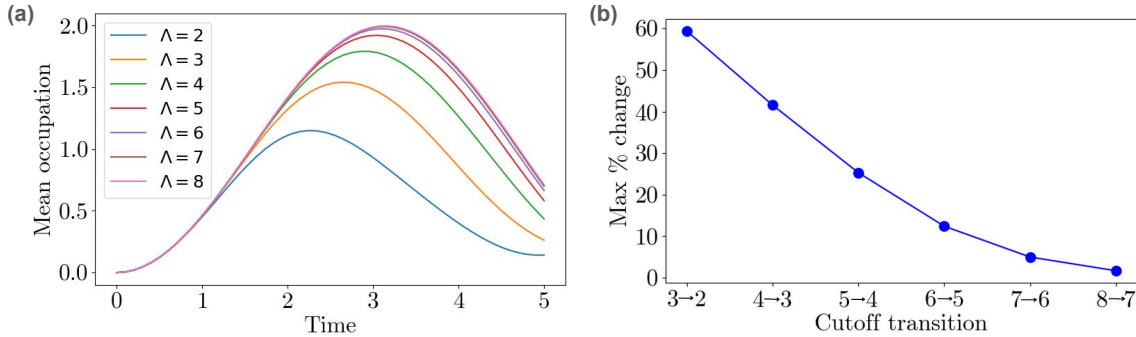

FIG. 4. (a) Mean boson occupations for mode 2 with varying  $\Lambda$ . (b) The variation in the mean boson occupation of mode 2 when the cutoff is decreased from  $\Lambda + 1$  to  $\Lambda$ . The variation is observed to diminish as  $\Lambda$  increases.

### B. Numerical emulation of the Trotter circuits

Simulations of Trotterized evolution were done using bosonic qiskit [2], an extension to the widely-used qiskit package that adds the capability of simulating bosonic degrees of freedom. Bosonic qiskit encodes the state of the boson using  $n$  qubits, where  $n$  is set by the user. As such, the highest occupation for a given boson will be  $2^n - 1$ . For all Trotterized simulations in the paper, we set  $n = 4$ .

- 
- [1] R. J. MacDonell, T. Navickas, T. F. Wohlers-Reichel, C. H. Valahu, A. D. Rao, M. J. Millican, M. A. Currington, M. J. Biercuk, T. R. Tan, C. Hempel, *et al.*, Chemical Science **14**, 9439 (2023).
  - [2] T. J. Stavenger, E. Crane, K. C. Smith, C. T. Kang, S. M. Girvin, and N. Wiebe, in *2022 IEEE High Performance Extreme Computing Conference (HPEC)* (IEEE, 2022) pp. 1–8.
